# Supplementary material for: Acceleration of relativistic beams using laser-generated terahertz pulses
Source: arXiv:1908.04055 source file (2019-08-12)
Supplement: Supplementary file 1 [file supplementary_info.pdf]

# Supplementary information

# Acceleration of relativistic beams using laser-generated terahertz pulses

M. T. Hibberd[1,2], A. L. Healy[1,3], D. S. Lake[1,4], V. Georgiadis[1,2], E. J. H. Smith[1,2], O. J. Finlay[1,4], T. H. Pacey[1,5], J. K. Jones[1,5], Y. Saveliev[1,5], D. A. Walsh[1,5], E. W. Snedden[1,5], R. B. Appleby[1,2], G. Burt[1,3], D. M. Graham[1,2] and S. P. Jamison[1,4]

[1]The Cockcroft Institute, Sci-Tech Daresbury, Keckwick Lane, Daresbury, Warrington WA4 4AD, UK.
[2]School of Physics and Astronomy & Photon Science Institute, The University of Manchester, Oxford Road, Manchester M13 9PL, UK.
[3]Department of Engineering, Lancaster University, Bailrigg, Lancaster LA1 4YW, UK.
[4]Department of Physics, Lancaster University, Bailrigg, Lancaster LA1 4YB, UK.
[5]Accelerator Science and Technology Centre, Science and Technology Facilities Council, Sci-Tech Daresbury, Keckwick Lane, Daresbury, Warrington WA4 4AD, UK.

## Waveguide dimensions

The dielectric-lined waveguide (DLW) assembly consisted of the DLW, a linearly tapered horn coupler (without a dielectric lining), and a detachable shelf with an aluminium mirror, as shown in Fig. S1a. The DLW assembly was manufactured in two parts, with the top and bottom sections joined together with the aid of alignment pins. The aluminium mirror had a 400 μm aperture for electron beam propagation and an attached 5 mm x 5 mm YAG screen, imaged by a camera for coarse electron beam alignment. Microscope images of the coupler entrance (Fig. S1b) and DLW exit (Fig. S1c) indicate the measured dimensions, with a 60 μm-thick fused-quartz dielectric lining the top and bottom of the waveguide.

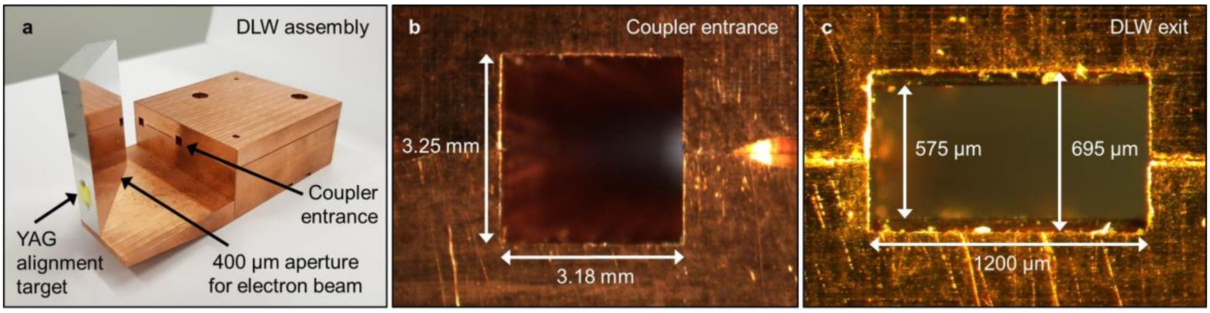


Fig. S1. **a,** Photograph of the complete DLW assembly. **b,c,** Microscope images of the (**b**) coupler entrance and (**c**) DLW exit.

## Waveguide dispersion

The dielectric lining in the waveguide modifies the dispersion relation from that of a hollow rectangular waveguide, acting to couple the typical transverse magnetic (TM) and electric (TE) modes into hybrid longitudinal section magnetic (LSM) modes. These modes enable propagation at phase velocities below the speed of light for matching to the particle velocity at a defined operating frequency of the DLW. The polarization and spatial profile of the driving THz electric field determines which mode is excited in the DLW, with $LSM_{11}$ being the first accelerating mode.

The dispersion relation of the $LSM_{11}$ mode [1] was numerically solved using the measured dimensions of the DLW (and a relative permittivity of $\varepsilon$ = 4 for the fused-quartz dielectric) to ascertain the longitudinal wavenumber ($\beta$) as a function of frequency, shown in Fig. S2a. At the

design frequency of 0.4 THz, the dispersion relation results in propagation at a phase velocity $v_p = 0.999c$ corresponding to the velocity of 35 MeV electrons, with a cut-off frequency at $f_c = 0.23$ THz. The phase and group velocity ($v_g$) of the $LSM_{11}$ mode are given in Fig. S2b and give a value of $v_g = 0.585c$ at 0.4 THz for this waveguide design.

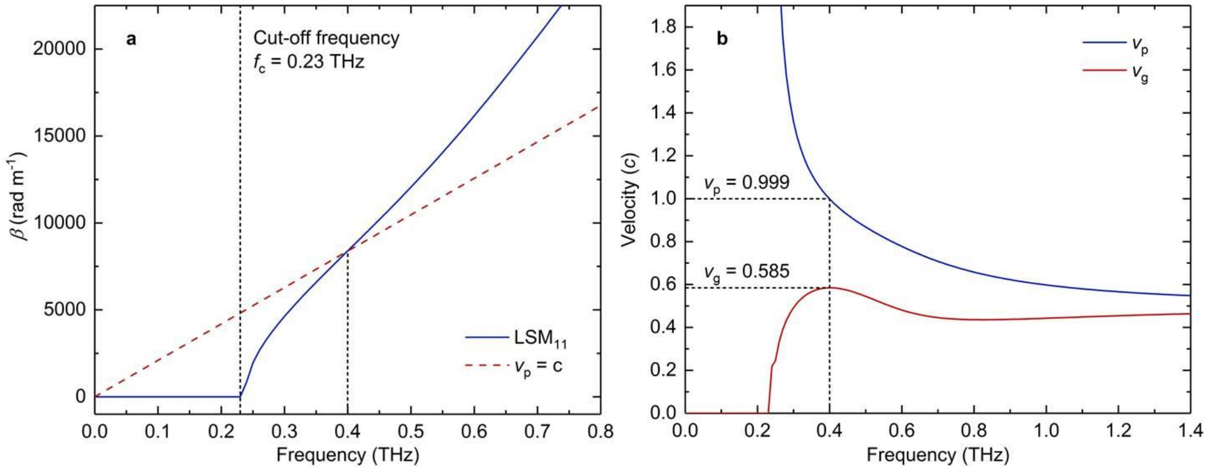


Fig. S2. **a,** Calculated dispersion relation for the $LSM_{11}$ mode of the DLW with the dashed line representing $v_p = c$. **b,** Calculated phase and group velocity of the $LSM_{11}$ mode as a function of frequency.

## Terahertz transmission measurements

Measurements of a broadband THz pulse transmitted through the DLW were performed to determine the cut-off frequency and dispersion of the DLW. The source was a combined spintronic THz emitter, consisting of two vertically stacked spintronic emitters with opposite ordering of the magnetic ($Co_{20}Fe_{60}B_{20}$) and non-magnetic (Pt) layers. This resulted in generation of opposite polarity THz radiation from the top and bottom halves of the combined source, creating a broadband quasi-$TEM_{01}$ mode similar to that produced by Cliffe *et al.* [2] and Hibberd *et al.* [3]. This quasi-$TEM_{01}$ mode was used to couple into the $LSM_{11}$ accelerating mode of the DLW and directly measure the mode properties. Electro-optic sampling measurements at the exit of the DLW are given in Fig. S3, showing the amplitude (Fig. S3a) and dispersion (Fig. S3b) of the transmitted THz pulse. In Fig. S3b, a cut-off frequency of approximately 0.25 THz was observed, consistent with the value predicted from the dispersion calculations in Fig. S2a.

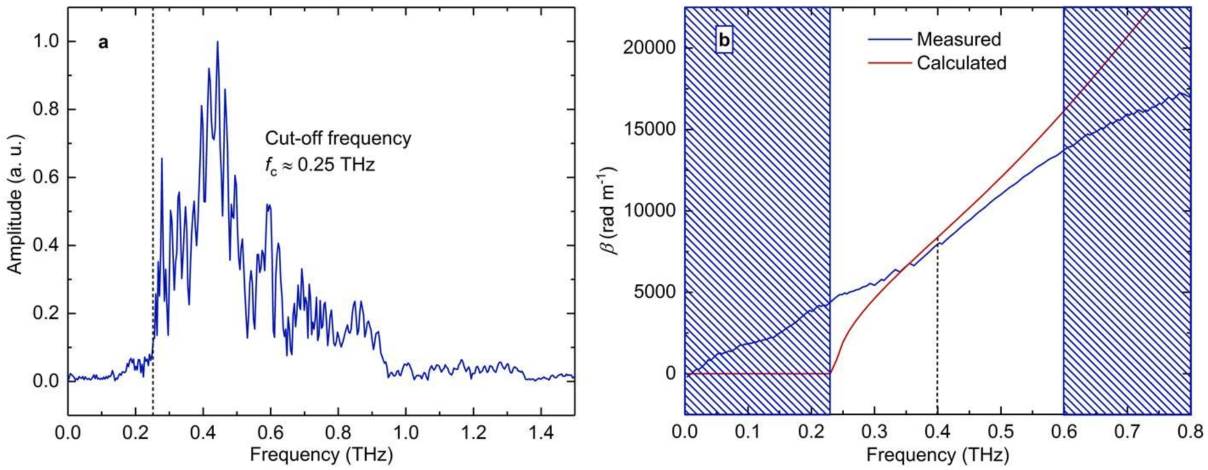


Fig. S3. **a,** THz frequency spectrum transmitted through the DLW and measured using a 500 µm-thick, (110)-cut ZnTe detection crystal at the exit of the DLW. **b,** Corresponding dispersion (shaded areas indicate regions of high phase uncertainty due to the low spectral amplitude) compared with calculated dispersion from Fig. S2a.

## Interaction length

The interaction length is typically defined by the length of the structure. However, the THz pulse duration, bandwidth and group-velocity walk-off limit the accelerating interaction length to less than the structure length. While the interaction length can be defined by simple expressions, derived for the phase and pulse slippage, these can underestimate the length of the interaction [1]. To determine the full extent of the interaction, the measured THz pulse was simulated inside the DLW structure using CST particle studio. As can be seen in Fig. S4, tracking an electron through the DLW reveals the total length of interaction is approximately 9 mm, although the acceleration decays with distance, with the FWHM of the interaction length occurring over 4.3 mm. The simulation also revealed that the peak longitudinal electric field on-axis at the DLW entrance was 2.2 times larger than the peak transverse electric field at the horn entrance.

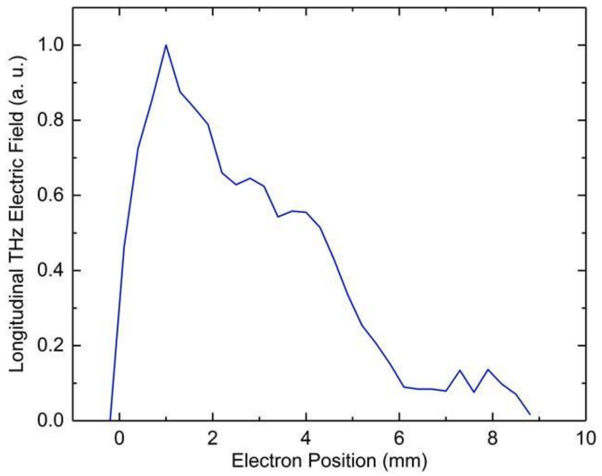


Fig. S4. Longitudinal accelerating electric field in the DLW experienced by a synchronous electron, simulated for the measured THz pulse in CST particle studio.

## References

[1] Healy, A. L., Burt, G. & Jamison, S. P. Electron-terahertz interaction in dielectric-lined waveguide structures for electron manipulation. *Nucl. Instr. Meth. Phys. Res. A* **909,** 199-203 (2018).

[2] Cliffe, M. J., Graham, D. M. and Jamison, S. P. Longitudinally polarized single-cycle terahertz pulses generated with high electric field strengths. *Appl. Phys. Lett.* **108**, 221102 (2016).

[3] Hibberd, M. T., Lake, D. S., Johansson, N. A. B., Thomson, T., Jamison, S. P. and Graham, D. M. Magnetic-field tailoring of the terahertz polarization emitted from a spintronic source. *Appl. Phys. Lett*. **114**, 031101 (2019).
